# Supplementary material for: Partially-Bright Triplet Excitons in Perovskite Nanocrystals
Source: arXiv:2002.08349 source file (2020-02-26)
Supplement: Supplementary file 1 [file SupplementalInfo.pdf]

# Supplemental Information for:

# Partially-Bright Triplet Excitons in Perovskite Nanocrystals

**Contents**


**I. Sample Synthesis and Characterization** 2

A. Preparation of Cs-Oleate Stock Solution 3

B. Synthesis of $CsPbI_3$ perovskite nanocrystals with Cs:Pb:I = 1:4.34:8.68 Molar Ratio 3

C. Transmission Electron Microscopy (TEM) 4

**II. Details of Experiment** 4

**III. Mapping Feynman Diagrams to Peaks in 2-D Spectra** 5

A. Third-Order Response Function 5

B. Phase-Matching 6

C. Double-Sided Feynman Diagrams 6

D. Equation Form of Diagrams 7

**IV. One-Quantum Lineshapes** 8

Time-Domain Signal 8

New Transform Axes 9

Shift and Projection 10

Inhomogeneous Limit 10

**V. Zero-Quantum Lineshapes** 11

**VI. One-Quantum Lineshape Fits** 12

A. Co-linear Spectrum Fits 12

B. Cross-linear Spectrum Fits 13

**VII. Co-Linear Zero-Quantum Spectra** 15

**References** 15


## I. SAMPLE SYNTHESIS AND CHARACTERIZATION

Synthesis of the nanocrystals used in this study follows the procedures detailed in [1, 2].

### A. Preparation of Cs-Oleate Stock Solution

80 mg of $Cs_2CO_3$ (0.5 mM $Cs^+$) was added to a 50 mL 2-neck round-flask, followed by addition of 1 mL of oleic acid and 7 mL of 1-octadecene. The flask was connected to a Schlenk line and vigorously stirred under vacuum at 100°C for 1 hour. After obtaining a transparent solution ($[Cs^+]$ = 0.06 mol/L), the system was maintained at 80°C under nitrogen flow to avoid the formation of a white precipitate.

### B. Synthesis of $CsPbI_3$ perovskite nanocrystals with Cs:Pb:I = 1:4.34:8.68 Molar Ratio

100 mg of $PbI_2$ (≈ 0.217 mM) was added to a 50 mL 3-neck round-flask, followed by the addition of 4.5 mL of 1-octadecene. The flask was connected to a Schlenk line and vigorously stirred under vacuum at 100°C for 30 min. Afterwards 1 mL of oleic acid and 0.5 mL of oleylamine was added, while keeping the reaction flask under vigorous stirring in vacuum at 100 °C until complete solubilization of the $PbI_2$, upon obtaining a transparent yellow solution. Prior to injection of the $Cs^+$ precursor, the temperatures of the $Pb^{2+}$ and $I^-$ precursor solutions were raised to 140°C under vigorous stirring and nitrogen flow, followed by swift injection of 0.8 mL of Cs-oleate stock solution. Formation of an intense red colloidal suspension of CsPbI3 nanocrystals was then observed. The suspension was immediately submerged in a cold water bath to cool down to room temperature for quenching nanocrystal growth.

The nanocrystals were cleaned by adding 15 mL of anhydrous methylacetate and centrifuged at 12000 rpm for 5 minutes. The supernatant was discarded and the precipitated nanocrystals were redispersed in anhydrous hexane.

### C. Transmission Electron Microscopy (TEM)

Transmission electron micrographs were acquired on the $CsPbI_3$ sample:

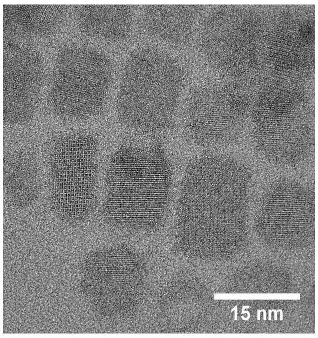


FIG. 1: Room-temperature TEM micrograph of $CsPbI_3$ nanocrystals.

100 nanocrystals were measured to obtain an average edge length 8.7 ± 2.6 nm.

## II. DETAILS OF EXPERIMENT

We use a Multi-Dimensional Optical Nonlinear Spectrometer (MONSTR) [3], which focuses three laser pulses onto the sample. The excitation pulses are of 90 fs duration at a 250 kHz repetition rate, and the excitation intensity of 5 W/cm$^2$ generates a predominately third-order response as verified by a power-dependence measurement of the generated transient four-wave-mixing signal. The emitted signal is then heterodyne detected [4] with a co-propagating local-oscillator pulse as a function of time delays $\tau$, $T$, and/or $t$ with sub-wavelength stability.

The sample studied is an ensemble of $CsPbI_3$ perovskite nanocrystals dispersed in heptomethylnonane and suspended in a copper sample holder with sapphire windows. The sample optical density is measured to be 0.3 at the room-temperature 1S exciton absorption peak.

## III. MAPPING FEYNMAN DIAGRAMS TO PEAKS IN 2-D SPECTRA

### A. Third-Order Response Function

The interpretation of 2-D spectra is performed through a perturbative expansion of the material polarization in response to a weak field. The third-order response may be written as:

$$P^{(3)}(t) \propto \int_0^\infty \int_0^\infty \int_0^\infty E(t-t_3)E(t-t_3-t_2)E(t-t_3-t_2-t_1)R(t_3,t_2,t_1)\mathrm{d}t_1\mathrm{d}t_2\mathrm{d}t_3 \quad (1)$$

where the times $t_1$, $t_2$, and $t_3$ are defined:

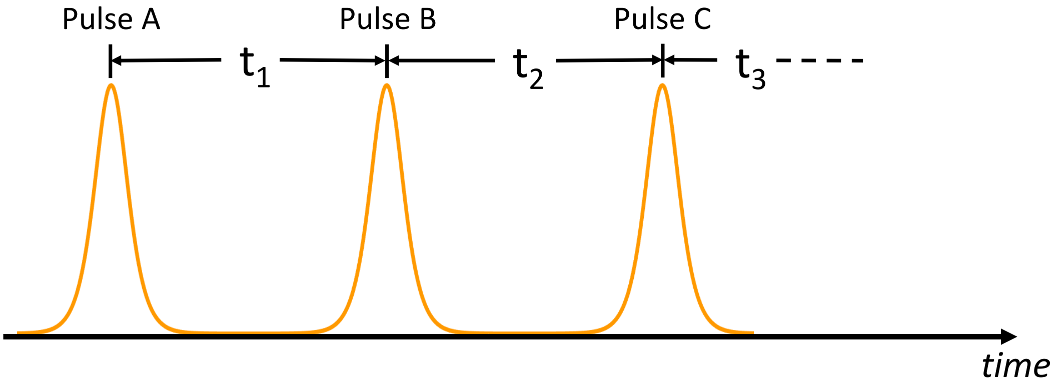


There is thus a direct correspondence between each field term in the third-order polarization and a single pulse in a three-pulse experiment. Note that what we denote $t_1$, $t_2$, and $t_3$ here are equivalent to the delays $\tau$, $T$, and $t$ respectively (as denoted in the main paper).

The response function $R(t_3,t_2,t_1)$ is defined by:

$$R^{(3)}(t_3,t_2,t_1) = -i\mathrm{Tr}\left\{\hat{\mu}(t_3+t_2+t_1),[\hat{\mu}(t_2+t_1),[\hat{\mu}(t_1),[\hat{\mu}(0),\rho(t_0)]]]\right\} \quad (2)$$

where $\rho(t_0)$ is the initial density matrix of the system (which we take to be the ground state density matrix $|g\rangle\langle g|$), Tr{...} denotes the trace operation and $\hat{\mu}(t)$ is the dipole operator in the interaction picture. We see that the response function is composed of three nested commutators, and thus contains 8 terms.

### B. Phase-Matching

We see in equation (1) that there are three fields that each may be written in complex form:

$$E(t) \propto \mathcal{E}(t) \left( e^{+i\omega t - i\mathbf{k}\cdot\mathbf{r} - i\phi} + e^{-i\omega t + i\mathbf{k}\cdot\mathbf{r} + i\phi} \right) \tag{3}$$

where $\omega$ and $\mathbf{k}$ are the angular frequency and wavevector that characterize the electromagnetic wave, and $\mathcal{E}(t)$ is the pulse envelope.

In equation (2), the dipole operators are written in the interaction picture. This means they involve both interactions via the dipole operator $\hat{\mu}$ **and** density matrix evolution at the transition frequency $\omega_{ij}$, where $|i\rangle$ and $|j\rangle$ are two states separated by the optical frequency we excite at. After taking into account both the optical field terms in equation (3) and the density matrix evolution terms, various terms will become negligible in the rotating wave approximation (RWA).

That is, for certain combinations $\pm\omega_A \pm \omega_B \pm \omega_C$ (and equivalently $\pm\mathbf{k}_A \pm \mathbf{k}_B \pm \mathbf{k}_C$), only certain terms of the nested commutator in equation (2) will be non-negligible. In our experiment, we isolate the polarization that radiates in the direction $\mathbf{k} = -\mathbf{k}_A + \mathbf{k}_B + \mathbf{k}_C$, and therefore isolate specific terms via *wave-vector selection.* The tedious process of calculating the explicit terms that survive the RWA may be considerably simplified by use of double-sided Feynman diagrams.

### C. Double-Sided Feynman Diagrams

As mentioned above, in our experiment we isolate the radiated signal in the $\mathbf{k} = -\mathbf{k}_A + \mathbf{k}_B + \mathbf{k}_C$ direction. Because of the minus sign in front of $\mathbf{k}_A$, we say that pulse $A$ is *conjugated*, while pulses B and C are *non-conjugated.* With these terms defined, we may construct the Feynman diagrams used to interpret the collected signal. An example diagram is shown:

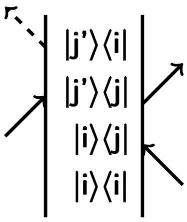

where $|i\rangle$ is lower in energy with respect to $|j\rangle$ and $|j'\rangle$. The states $|i\rangle$ and $|j\rangle/|j'\rangle$ are separated by $\hbar\omega_{ij}/\hbar\omega_{ij'}$, where $\omega_{ij}/\omega_{ij'}$ are optical frequencies we excite at.

The diagram may be constructed as follows:

1. Time increases from the bottom of the diagram going up.
2. The density matrix element at the bottom $|i\rangle\langle i|$ is the initial density matrix of the system and must be a population state.
3. Pulse interactions are represented by arrows; arrows pointing (out)inwards cause (de)excitation of either the Ket or Bra, depending on the side on which the arrow is placed.
4. Ordering of the arrows going from the bottom upwards follows the time-ordering of the pulses in experiment.
5. Conjugated pulses are represented by left-pointing arrows, and non-conjugated pulses are represented by right-pointing arrows.
6. For a $n$-order process, there are $n$ arrows and $n$ density matrix elements after the initial density matrix $|i\rangle\langle i|$.

All diagrams that contribute to the measured signal may be found by taking all combinations of density matrix elements and arrows on either side that satisfy the above rules.

### D. Equation Form of Diagrams

We now demonstrate how one may write down the relevant third-order polarization terms directly from the double-sided Feynman diagrams. We show the example diagram from before and its corresponding equation:

Here, we've highlighted each density matrix element and its corresponding terms in equation form. We see that the density matrix element induced by each pulse will oscillate at the difference frequency of the two states composing the Bra and Ket for a time $t_i$ until the next excitation pulse or detection. For simplicity, we've included the Markovian dephasing terms $\Gamma_{ij}$, which correspond to either coherence dephasing (if $i \neq j$) or population relaxation

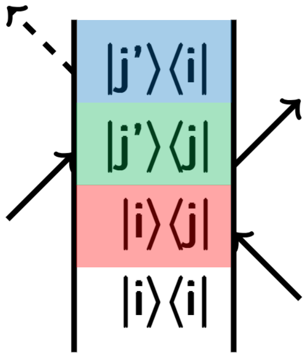


$$e^{-i(\omega_{ii}-\omega_{ji})t_1} e^{-i(\omega_{j'i}-\omega_{ji})t_2} e^{-i(\omega_{j'i}-\omega_{ii})t_3} e^{-\Gamma_{ji}t_1} e^{-\Gamma_{j'j}t_2} e^{-\Gamma_{j'i}t_3}$$

(if $i = j$). If the coherences evolve outside of the Markovian dephasing regime, we replace these terms by those of the form $e^{-g(t)}$, where $g(t)$ is the lineshape function characterizing the system-bath interaction.

## IV. ONE-QUANTUM LINESHAPES

We show straightforward extensions of the procedure outlined by Siemens et al. [5] to fit lineshapes of sidebands in one-quantum and zero-quantum spectra.

### Time-Domain Signal

We consider the case of a rephasing signal resulting from excitation and emission frequencies $\omega_1$ and $\omega_2$ respectively (ignoring dynamics during $T$), and assume perfectly correlated inhomogeneous broadening between the two transitions with dephasing rates $\gamma_1$ and $\gamma_2$:

$$\begin{aligned} s(t,\tau) &= \Theta(t)\Theta(\tau)e^{-\gamma_1\tau}e^{-\gamma_2 t}\int e^{-i[(\omega_1+\Delta\omega)\tau-(\omega_2+\Delta\omega)t]}e^{-\frac{\Delta\omega^2}{2\sigma^2}}d\Delta\omega \\ &= \Theta(t)\Theta(\tau)e^{-\gamma_1\tau}e^{-\gamma_2 t}e^{-i\omega_1\tau}e^{+i\omega_2 t}\,\mathcal{F}\left\{e^{-\frac{\Delta\omega^2}{2\sigma^2}}\right\}\Big|_{t-\tau} \\ &\propto \Theta(t)\Theta(\tau)e^{-\gamma_1\tau}e^{-\gamma_2 t}e^{-i\omega_1\tau}e^{+i\omega_2 t}e^{-\frac{\sigma^2}{2}(t-\tau)^2} \end{aligned} \tag{4}$$

Defining the new time variables:

$$t' = \frac{1}{2}(t+\tau) \qquad \tau' = \frac{1}{2}(t-\tau) \tag{5}$$

We recast the time-domain signal:

$$s(t',\tau') = \Theta(t'+\tau')\Theta(t'-\tau')e^{-\gamma_1(t'-\tau')}e^{-\gamma_2(t'+\tau')}e^{-i\omega_1(t'-\tau')}e^{+i\omega_2(t'+\tau')}e^{-2\sigma^2\tau'^2} \tag{6}$$

**New Transform Axes**

It is important to determine the specific axes that the new time-variables result in after Fourier transform. Writing out the original transform:

$$f(t,\tau) = \iint e^{-i(\omega_t t+\omega_\tau \tau)} f(\omega_t,\omega_\tau)d\omega_\tau d\omega_t \tag{7}$$

In terms of the new time variables:

$$\begin{aligned} f(t',\tau') &= \iint e^{-i[\omega_t(t'+\tau')+\omega_\tau(t'-\tau')]} f(\omega_t,\omega_\tau)d\omega_\tau d\omega_t \\ &= \iint e^{-i[(\omega_t+\omega_\tau)t'+(\omega_t-\omega_\tau)\tau']} f(\omega_t,\omega_\tau)d\omega_\tau d\omega_t \end{aligned}$$

We see that the natural conjugate variables for $t'$ and $\tau'$ are:

$$\omega_{t'} = \omega_t + \omega_\tau \qquad \omega_{\tau'} = \omega_t - \omega_\tau \tag{8}$$

or equivalently:

$$\omega_t = \omega_{t'} + \omega_{\tau'} \qquad \omega_\tau = \omega_{t'} - \omega_{\tau'} \tag{9}$$

NOTE: In the rephasing pulse sequence, $\omega_\tau$ is <u>negative</u>.

Using the Jacobian of our variable transformation:

$$J = \begin{vmatrix} \frac{d\omega_t}{d\omega_{t'}} & \frac{d\omega_t}{d\omega_{\tau'}} \\ \frac{d\omega_\tau}{d\omega_{t'}} & \frac{d\omega_\tau}{d\omega_{\tau'}} \end{vmatrix} = -1 - 1 = -2 \tag{10}$$

We change the variables of integration:

$$f(t',\tau') = 2\iint e^{-i(\omega_{t'}t'+\omega_{\tau'}\tau')} f(\omega_{t'},\omega_{\tau'})d\omega_{\tau'} d\omega_{t'} \tag{11}$$

**Shift and Projection**

We now shift the signal to the origin in our $\tau'$ and $t'$ coordinates via multiplication by $e^{+i\omega_1(t'-\tau')\tau'}e^{-i\omega_2(t'+\tau')}$:

$$s_{origin}(t',\tau') = \Theta(t'+\tau')\Theta(t'-\tau')e^{-\gamma_1(t'-\tau')}e^{-\gamma_2(t'+\tau')}e^{-2\sigma^2\tau'^2} \tag{12}$$

The projections along $t'$ and $\tau'$ are then:

$$s_{proj,t'} = \int_{-\infty}^{\infty} s_{origin}(t',\tau')d\tau' = e^{-(\gamma_1+\gamma_2)t'}\int_{-t'}^{t'} e^{(\gamma_1-\gamma_2)\tau'}e^{-2\sigma^2\tau'^2}d\tau' \tag{13}$$

$$s_{proj,\tau'} = \int_{-\infty}^{\infty} s_{origin}(t',\tau')dt' = e^{(\gamma_1-\gamma_2)\tau'}e^{-2\sigma^2\tau'^2}\int_{|\tau'|}^{\infty} e^{-(\gamma_1+\gamma_2)t'}dt' \tag{14}$$

where the Heaviside functions are accounted for by change of integration limits.

**Inhomogeneous Limit**

In the inhomogeneous limit ($\sigma \gg \gamma_1, \gamma_2$) the signal decays along $\tau'$ much faster than along $t'$. In the integral along $\tau'$ we can approximate the gaussian portion of the kernel as a delta function. In the integral along $t'$, we can approximate the lower limit as 0. These two limits give:

$$s_{proj,t'} = e^{-(\gamma_1+\gamma_2)t'}\int_{-t'}^{t'} e^{(\gamma_1-\gamma_2)\tau'}\delta(\tau')d\tau' = e^{-(\gamma_1+\gamma_2)t'}\Theta(t') \tag{15}$$

$$s_{proj,\tau'} = e^{(\gamma_1-\gamma_2)\tau'}e^{-2\sigma^2\tau'^2}\int_{0}^{\infty} e^{-(\gamma_1-\gamma_2)t'}dt' = e^{(\gamma_1-\gamma_2)\tau'}e^{-2\sigma^2\tau'^2} \tag{16}$$

which then give the frequency domain lineshapes in the inhomogeneous limit:

$$S_{slice}(\omega_{t'}) \propto \frac{1}{(\gamma_1+\gamma_2)+i\omega_{t'}} \qquad \text{(Cross-Diagonal)} \tag{17}$$

$$S_{slice}(\omega_{\tau'}) \propto e^{-\frac{\omega_{\tau'}^2}{8\sigma^2}} \qquad \text{(Diagonal)} \tag{18}$$

where we've assumed $\gamma_1 - \gamma_2 \ll \sigma$.

## V. ZERO-QUANTUM LINESHAPES

The lineshapes of a zero-quantum spectrum can be derived by the same method, with inclusion of an intermediate zero-quantum coherence with a dephasing rate of $\gamma_T$:

$$\begin{aligned}
s(t,T,\tau) &= \Theta(t)\Theta(T)\Theta(\tau)e^{-\gamma_1\tau}e^{-\gamma_2 t}e^{-\gamma_T T}\int e^{-i[(\omega_1+\Delta\omega)\tau-(\omega_2+\Delta\omega)t]}e^{i(\omega_2-\omega_1)T}e^{-\frac{\Delta\omega^2}{2\sigma^2}}d\Delta\omega \\
&= \Theta(t)\Theta(T)\Theta(\tau)e^{-\gamma_1\tau}e^{-\gamma_2 t}e^{-\gamma_T T}e^{+i(\omega_2-\omega_1)T}e^{-i\omega_1\tau}e^{+i\omega_2 t}\int e^{+i\Delta\omega(t-\tau)}e^{-\frac{\Delta\omega^2}{2\sigma^2}}d\Delta\omega \\
&= \Theta(t)\Theta(T)\Theta(\tau)e^{-\gamma_1\tau}e^{-\gamma_2 t}e^{-\gamma_T T}e^{+i(\omega_2-\omega_1)T}e^{-i\omega_1\tau}e^{+i\omega_2 t}\ \mathcal{F}\left\{e^{-\frac{\Delta\omega^2}{2\sigma^2}}\right\}\Bigg|_{t-\tau} \\
&= \Theta(t)\Theta(T)\Theta(\tau)e^{-\gamma_1\tau}e^{-\gamma_2 t}e^{-\gamma_T T}e^{+i(\omega_2-\omega_1)T}e^{-i\omega_1\tau}e^{+i\omega_2 t}\left[e^{-\frac{\sigma^2}{2}t'^2}\right]_{t'=t-\tau} \\
&= \Theta(t)\Theta(T)\Theta(\tau)e^{-\gamma_1\tau}e^{-\gamma_2 t}e^{-\gamma_T T}e^{+i(\omega_2-\omega_1)T}e^{-i\omega_1\tau}e^{+i\omega_2 t}e^{-\frac{\sigma^2}{2}(t-\tau)^2}
\end{aligned} \tag{19}$$

Shift frequency domain peak to origin:

$$\begin{aligned}
s_{origin}(t,T,\tau) &= s(t,T,\tau)e^{-i(\omega_2-\omega_1)T}e^{-i\omega_2 t} \\
&= \Theta(t)\Theta(T)\Theta(\tau)e^{-\gamma_1\tau}e^{-\gamma_2 t}e^{-\gamma_T T}e^{-i\omega_1\tau}e^{-\frac{\sigma^2}{2}(t-\tau)^2}
\end{aligned} \tag{20}$$

Project onto $T$ axis:

$$\begin{aligned}
s_{proj}(T) &= \int_{-\infty}^{\infty} s_{origin}(t,T,\tau)dt \\
&= \Theta(t)\Theta(T)\Theta(\tau)e^{-\gamma_1\tau}e^{-\gamma_T T}e^{-i\omega_1\tau}\int_0^{\infty} e^{-\gamma_2 t}e^{-\frac{\sigma^2}{2}(t-\tau)^2}dt \\
&= \Theta(t)\Theta(T)\Theta(\tau)e^{-(\gamma_1+\gamma_2)\tau}e^{-\gamma_T T}e^{-i\omega_1\tau}\int_{-\tau}^{\infty} e^{-\gamma_2 t'}e^{-\frac{\sigma^2}{2}t'^2}dt'
\end{aligned} \tag{21}$$

In the inhomogeneous limit:

$$s_{proj}(T) = \Theta(t)\Theta(T)\Theta(\tau)e^{-(\gamma_1+\gamma_2)\tau}e^{-\gamma_T T}e^{-i\omega_1\tau} \tag{22}$$

which gives the lineshape:

$$\begin{aligned}
S_{slice}(\omega_T) &= \Theta(t)\Theta(\tau)e^{-(\gamma_1+\gamma_2)\tau}e^{-i\omega_1\tau}\mathcal{F}\left\{e^{-\gamma_T T}\Theta(T)\right\} \\
&\propto \Theta(t)\Theta(\tau)e^{-(\gamma_1+\gamma_2)\tau}e^{-i\omega_1\tau}\frac{1}{\gamma_T - i\omega_T}
\end{aligned} \tag{23}$$

## VI. ONE-QUANTUM LINESHAPE FITS

The lineshapes observed in the obtained one-quantum spectra, especially on the $\Delta E < 0$ side of each spectra, exhibit lineshapes distorted by vibrational coupling that deviate from ideal summations of Lorentzians. We thus fit the co-linear and cross-linear lineshapes with symmetric complex Lorentzian peaks, but only on the $\Delta E \geq 0$ side.

### A. Co-linear Spectrum Fits

To investigate the dependence of parameters on nanocrystal size, we fit cross-diagonal slices centered at various slice positions $|\hbar\omega_\tau| = |\hbar\omega_t|$:

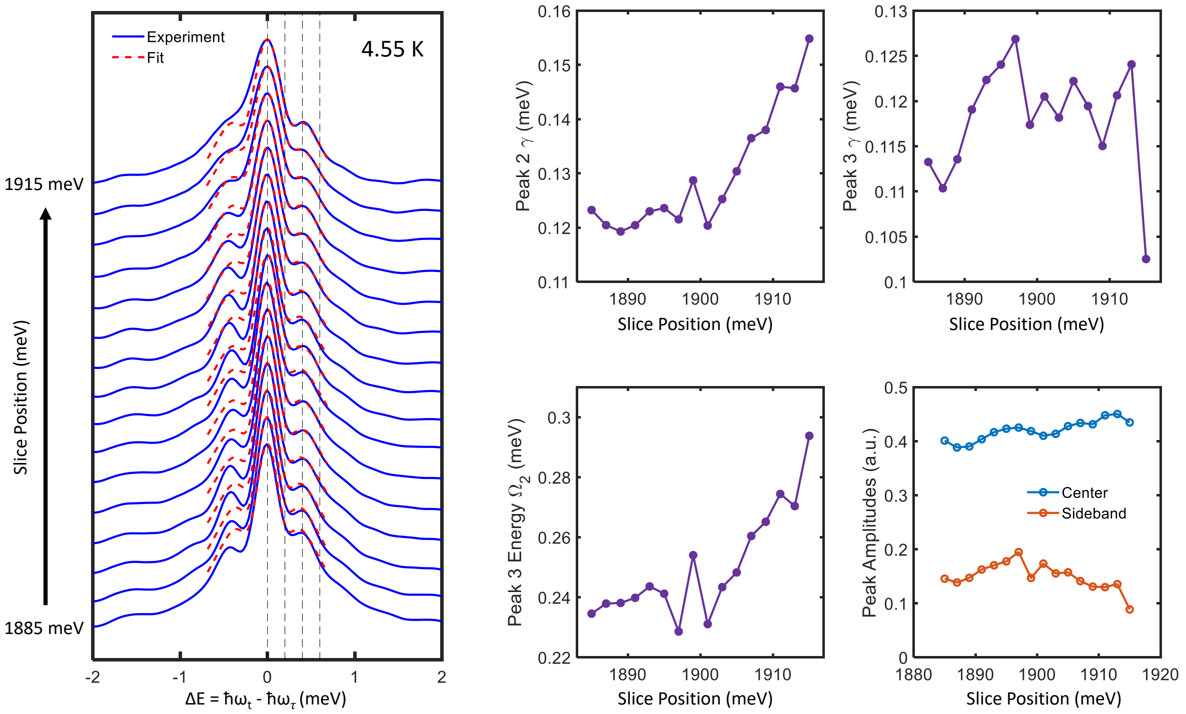


FIG. 2: Left: The slices from a co-linear one-quantum spectrum at 4.55 K are plotted as blue curves, with their corresponding fitted lineshapes overlayed as dashed red lines. Right: Fitted parameters are plotted as a function of slice position.

The slices are fitted in the range $0 \leq \Delta E \leq 0.7$ meV to three complex Lorentzians, where the sidebands are shifted in phase by $\frac{\pi}{2}$ to achieve the correct lineshapes.

### B. Cross-linear Spectrum Fits

Just as with the co-linear spectrum, we fit cross-diagonal slices centered at various slice positions $|\hbar\omega_\tau| = |\hbar\omega_t|$:

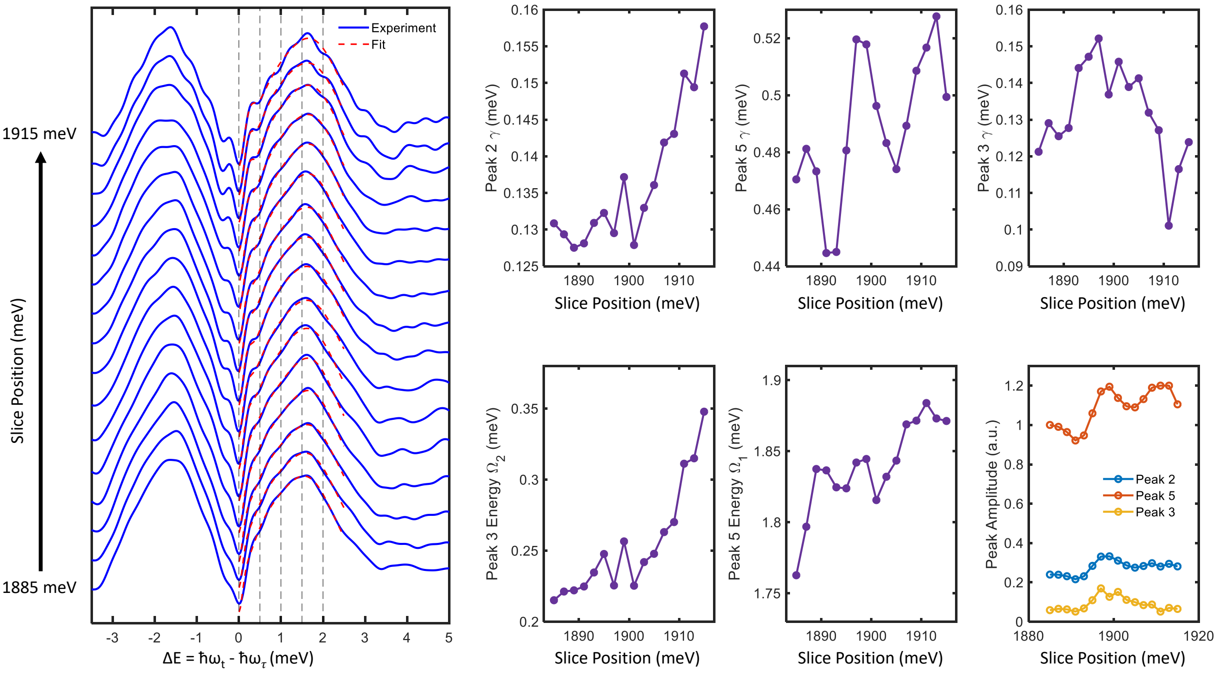


FIG. 3: Left: The slices from cross-linear one-quantum spectra are plotted as blue curves, with their corresponding fitted lineshapes overlayed as dashed red lines. Right: Fitted parameters are plotted as a function of slice position.

The slices are fitted in the range $0 \leq \Delta E \leq 2.5$ meV to five complex Lorentzians, where all four sidebands are shifted in phase by $\pi/2$ to achieve the correct lineshapes. To explore the possibility of a weak, third sideband at energy $\Delta E = \Omega_1 + \Omega_2$, corresponding to absorption and emission involving the states $|\psi_x\rangle$ and $|\psi_z\rangle$, we attempted to fit the above lineshapes with an additional two Lorentzian peaks. However, no reasonable fits were found possible.

From the fitted peak linewidths, we can extract the dephasing rates of the triplet state manifold $\gamma_x, \gamma_y$, and $\gamma_z$ as described in the main text:

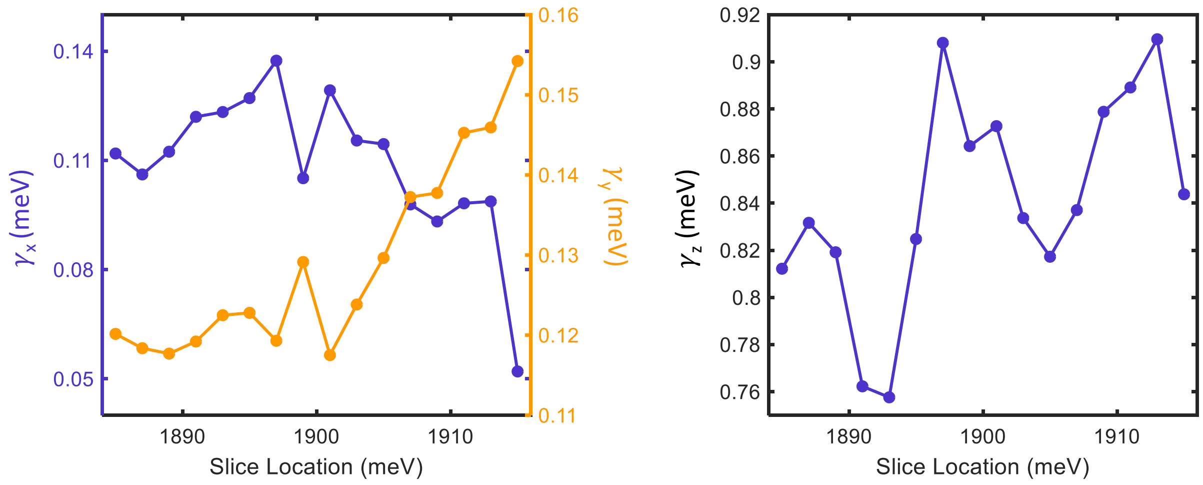


FIG. 4: Extracted dephasing rates of each triplet state transition.

While $\gamma_x$ does not exhibit a clear monotonic increase or decrease with changing size, $\gamma_y$ sharply increases at a slice position of around 1900 meV. This indicates that, within the size-distribution probed by our laser bandwidth, $|\psi_y\rangle$ becomes degenerate with $|\psi_d\rangle$ at an energy gap of around 1900 meV and becomes increasingly higher in energy at larger slice positions. A more statistically comprehensive study is needed to draw firm quantitative conclusions.

## VII. CO-LINEAR ZERO-QUANTUM SPECTRA

Zero-quantum spectra were acquired with a co-linear (HHHH) excitation scheme:

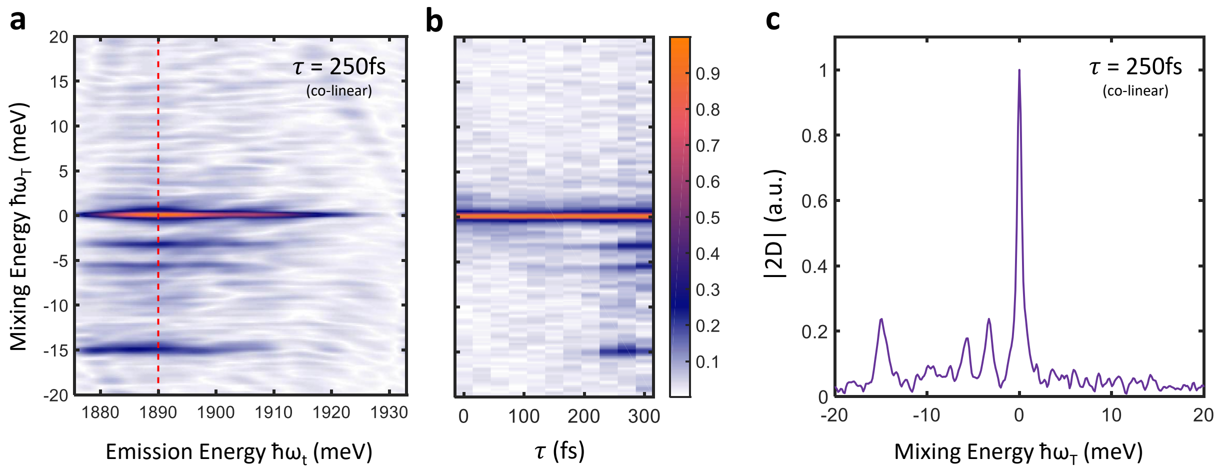


FIG. 5: (a) Zero-quantum spectra taken with co-linear excitation at $\tau = 250$ fs. (b) Evolution of normalized slices taken at $\hbar\omega_t = 1890$ meV (indicated by the dashed red line in figure a). (c) Normalized cross-slice taken at $\tau = 250$ fs and $\hbar\omega_t = 1890$ meV (indicated by the dashed red line in figure a).

No inter-triplet coherences were observed, which are expected to be symmetric in positive and negative mixing energy due to their electronic origin. However, multiple negative mixing energy sidebands appear with increasing delay $\tau$, which we attribute to electronic-vibrational coupling and discuss in a separate paper.


[1] L. Protesescu, S. Yakunin, M. I. Bodnarchuk, F. Krieg, R. Caputo, C. H. Hendon, R. X. Yang, A. Walsh, and M. V. Kovalenko, Nano Letters **15**, 3692 (2015), ISSN 1530-6984, URL `https://doi.org/10.1021/nl5048779`.

[2] L. Protesescu, S. Yakunin, S. Kumar, J. Bär, F. Bertolotti, N. Masciocchi, A. Guagliardi, M. Grotevent, I. Shorubalko, M. I. Bodnarchuk, et al., ACS Nano **11**, 3119 (2017), ISSN 1936-0851, URL `https://doi.org/10.1021/acsnano.7b00116`.

[3] A. D. Bristow, D. Karaiskaj, X. Dai, T. Zhang, C. Carlsson, K. R. Hagen, R. Jimenez, and S. T. Cundiff, Review of Scientific Instruments **80**, 073108 (2009), ISSN 0034-6748, URL `https:`

//doi.org/10.1063/1.3184103.

[4] L. Lepetit, G. Chériaux, and M. Joffre, Journal of the Optical Society of America B **12**, 2467 (1995), URL http://josab.osa.org/abstract.cfm?URI=josab-12-12-2467.

[5] M. E. Siemens, G. Moody, H. Li, A. D. Bristow, and S. T. Cundiff, Optics Express **18**, 17699 (2010), URL http://www.opticsexpress.org/abstract.cfm?URI=oe-18-17-17699.
